# Supplementary material for: Butterfly-Core Community Search over Labeled Graphs
Source: arXiv:2105.08628 source file (2021-05-20)
Supplement: Supplementary file 1 [file sec-appendix.tex]

%%
%% If your work has an appendix, this is the place to put it.
% \appendix
In our experiments, all the algorithms were implemented with C++ and conducted on a Linux Server with Intel Xeon CPU $E5-2620$ ($2.00$ GHz) and $65$ GB main memory.

\begin{table}[th]
\centering
\small
\vspace{-0.2cm}
\caption{Network statistics $(K = 10^3$ and $M = 10^6)$.}
\label{snap}
\vspace{-0.2cm}
\begin{tabular}{ l|rrrr }
\hline
{\bf Network} & $|V_G|$ & $|E_G|$ & $k_{max}$ & $d_{max}$  \\
 \hline
%Facebook  & 4\bf{K} & 88\bf{K} \\
Amazon  & 335\bf{K} & 926\bf{K} & 6 & 549\\
DBLP  & 317\bf{K} & 1\bf{M} & 113 & 342\\
Youtube & 1.1\bf{M} & 3\bf{M} & 51 & 28,754\\
LiveJournal & 4\bf{M} & 35\bf{M} & 360 &14,815\\
Orkut & 3.1\bf{M} & 117\bf{M} & 253 & 33,313\\ \hline
\end{tabular}
\vspace{-0.2cm}
\end{table}

\subsection*{Experimental Setup}
Our experiments are based on $5$ public real-world networks available from SNAP, namely Amazon, Dblp, Youtube, LiveJournal and Orkut, where all networks are treated as undirected. All the networks contain $5,000$ top-quality ground-truth communities. The network statistics are shown in Table~\ref{snap}.

\vspace{-0mm}
\spara{Network Construction.} Indeed, the nodes on the above original network do not have labels and there may not be edges across two communities. Therefore, we added new information for the network to fit our problem in the following steps:
\squishlisttight
\vspace{-1mm}
\item \spara{Add node labels}. We split the \textbf{w}hole \textbf{g}round \textbf{t}ruth \textbf{c}ommunities (wgtc) by communities into $t$ parts, assigning all the nodes in each part with one label. Here we set $t = 2$ which is the most challenging case when the size of the subgraph of one label is maximized. Since one node may have more than one community, if these communities appear in different parts, the nodes label will be randomly assigned. There are also very less nodes on the graph (less than $5\%$) have no communities whose labels are also randomly assigned. The community label is dominated by the majority label of its nodes.

\vspace{-1mm}
\item \spara{Generate qualified query pairs for test}. We selected the evaluated query pairs from the nodes shown in the \textbf{t}op \textbf{5}k \textbf{c}ommunities (t5c). We iterated the nodes in t5c and then picked out the nodes that have and only have one community in wgtc, generating the node set $S$. We then generate the node pairs from $S$ by picking any two nodes with different labels.

\vspace{-1mm}
\item \spara{Add cross edges between test communities}. We listed the test communities containing the nodes in $S$ and group these communities by their labels, the generation way of $S$ guarantees there is only one community including each node in $S$ and it is a top 5k community. For these communities with different labels, we randomly added ``edges ratio'' = 10\% cross edges into two communities.
\end{list}

\spara{Metric.}
For evaluating efficiency, we report the running time in seconds. We treat the running time of a query as infinite if it exceeds $30$ minutes. In addition, to evaluate the quality of the detected butterfly-core community, we implemented two classical community search methods: 1) $k$-core, which finds the dense subgraph where the degree of each node is no less than $k$; and 2) $k$-truss, where each edge has a support no less than $k - 2$, for both methods we add the same minimize diameter constraint. We test the datasets with ground-truth, and show the F1-score to measure the alignment between a discovered community $C$ and a ground-truth community $\hat{C}$. Here, F1 is defined as $F1(C, \hat{C}) = \frac{2·prec(C, \hat{C})·recall(C, \hat{C})}{prec(C, \hat{C}) + recall(C, \hat{C})}$ where $prec(C, \hat{C}) = \frac{|C \cap \hat{C}|}{|C|}$ is precision and $recall(C, \hat{C}) = \frac{|C \cap \hat{C}|}{|\hat{C}|}$ is recall.

\spara{Query pairs parameters.}
Two parameters, degree rank $Q_d$ and inter-distance $l$ are varied for selecting different sets of query nodes. Here, $Q_d$ is the degree rank of query nodes. We sorted all vertices in ascending order of their degrees in a network. A node is regarded to be with degree rank of $X\%$, if it has top highest $X\%$ degree in the network. The default value of $Q_d$ is $80\%$, which means that a query node has degree higher than the degree of $80\%$ nodes in the whole network. The inter-distance $l$ is the inter-distance between two query nodes. The default $l = 1$ indicates that the two query nodes are directly connected in the network. In summary, the default value of $Q_d$ is $80\%$ and the default distance $l$ is $l = 1$.

\spara{Model Parameters setting.}
For all the butterfly-core based models, i.e., BD, BD++ and LBCC++, we set $k_1$ and $k_2$ as the maximum core value of query nodes $q_l$ and $q_r$ could reach respectively. Note that this setting may not reach the best F1-score but it is reasonable for the users convenience especially when the users have no sense about the graph or query nodes. For $b$, we set $b = 1$. For LBCC, we select $\gamma_1 = 0.5$ and $\gamma_2 = 0.5$. For the baselines, we set $k$-core model with $k = 3$ and $k$-truss model with $k = 5$.
